# Supplementary material for: Flying Hand: End-Effector-Centric Framework for Versatile Aerial Manipulation Teleoperation and Policy Learning
Source: arXiv:2504.10334 source file (2025-04-14)
Supplement: Supplementary file 1 [file 99Appendix.tex]

\section*{Appendix}

\subsection{Disturbance Analysis}

We visualized the external wrench $\tau_{\text{ext}}$ on the base and the L1 estimation. The interaction force is within $5\ \text{N}$ and the torque within $1.4\ \text{Nm}$.
Fig.~\ref{fig: l1_disturbance} shows model uncertainties along the base $x$ (red), $z$ (blue) and $\theta_{pitch}$ (green), respectively. The uncertainties arise from inaccurate thrust gain and hovering thrust bias. Shaded areas indicate obvious interaction torque in base pitch resulting from arm motion.

Besides, the stability and robustness of the L1 controller under disturbances and state estimation inaccuracies for UAV systems are thoroughly analyzed theoretically in \citep{hovakimyan2010ℒ1} and extensively validated experimentally in \citep{gregory2009l1, wu2025l1}.

\begin{figure}[h]
    \centering
    \includegraphics[width=1.0\linewidth]{Figure/l1_dist_analysis.pdf}
    \caption{(a). Arm joint angles (b). Disturbance of $x$, $z$, and $\theta_{pitch}$}
    \label{fig: l1_disturbance}
\end{figure}

\subsection{Broader comparison with other works}

We replaced the IK with Direct Force Feedback Control (DFFC) for a more convincing baseline. DFFC calculates the desired EE acceleration from tracking errors and distributes control inputs to the base and arm. DFFC reduces the tracking error from $8.97\pm 0.79$ cm to $7.35\pm 0.51$ cm compared with the IK baseline. However, reactive control methods still have delays relative to predictive control methods, as shown by the phase lag of the orange line in Fig.~\ref{fig: tracking_DFFC}.

\begin{figure}[h]
    \centering
    \includegraphics[width=0.95\linewidth]{Figure/fig1_plot_enhance.pdf}
    \caption{EE tracking performance comparison of MPC and DFFC}
    \label{fig: tracking_DFFC}
\end{figure}

\subsection{Policy Learning with Less Accurate State Estimation}

In this work, we use a motion capture system to get the state estimation of the drone itself and further get the state estimation of the end-effector using proprioception information by forward kinematics. However, in more realistic scenarios like the outdoor environment, the high-precision motion capture system may not be applicable, and it further challenges the policy learning. To simulate this, we further evaluate the simulated peg-in-hole task with $1$ cm state estimation noise, an achievable precision with an RTK GPS in the real world \citep{feng2008gps}. It still achieved a $42\%$ successful rate with a limited 5k training epochs, proving the potential to deploy our system in outdoor environments without a motion capture system.
